# Supplementary material for: GC-Bench: An Open and Unified Benchmark for Graph Condensation
Source: arXiv:2407.00615 source file (2024-11-21)
Supplement: Supplementary file 1 [file 0_notations.tex]

\section{Notations}\label{sec:notation}
\setcounter{table}{0}
\setcounter{footnote}{0}
\setcounter{figure}{0}
\setcounter{equation}{0}

\begin{table}[htbp]
\vspace{-0.5em}
\label{tab:notation}%
\resizebox{\linewidth}{!}{
  \centering
    \begin{tabular}{cl}
    \toprule
    \textbf{Notations} & \multicolumn{1}{c}{\textbf{Descriptions}} \\
    \midrule
    $\mathbf{DG} = \{ \mathcal{G} \}_{t=1}^{T}$    & Dynamic graph (a set of $T$ discrete graph snapshots) \\
    $\mathcal{G} = (\mathcal{V}, \mathcal{E})$    & Graph with the node set $\mathcal{V}$ and edge set $\mathcal{E}$ \\
    $\mathcal{G}^t = (\mathcal{V}^t, \mathcal{E}^t)$ & Graph snapshot at time $t$ \\
    $\mathbf{X}^{t}$, $\mathbf{A}^t$ & Node features matrix and adjacency matrix of a graph at time $t$ \\
    $\mathbf{x}_v^{t}$, $\mathbf{A}_{(u,v),k}^t$ &  Node features and edge weights of $(u,v)$ under $\mathbf{e}_k$\\
    $\mathcal{G}^{1:t}$, $\mathcal{Y}^{t}$, $\mathbf{G}^{1:t}$, $\mathbf{Y}^{t}$ & Graph trajectory, labels and their corresponding random variables \\
    $\mathbf{e}$, $\mathbf{e}_i$, $\mathbf{E}$ & Latent environments and their support\\
    $\mathbf{z}_{v,k}^{t}$, $\mathbf{z}_{v}^{\mathbf{e},t}$, $\mathbf{z}_{v}^{\mathbf{e}}$ & Node representations under $\mathbf{e}_k$, at time $t$ and at overall time slices\\
    $\mathbf{z}$, $\mathbf{y}$ & Observed environment sample with its label\\
    $d$, $d^{\prime}$ & Dimension for $\mathbf{x}_v^t$ and $\mathbf{z}_{v,k}^t$, respectively\\
    $K$ & Number of underlying environments (number of convolution channel)\\
    $f(\cdot)$, $w(\cdot)$, $g(\cdot)$ & Model, encoder, and the link predictor\\
    $\ell(\cdot)$ & The loss function\\
    $q_\phi$, $p_\omega$ & The prior distribution and variational distribution of environments\\
    $\mathbb{I}^\star(\cdot)$, $\mathbb{I}(\cdot)$ & Invariant pattern recognition function and its implementation\\
    $\mathcal{P}_\mathbf{e}^I$, $\mathcal{P}_\mathbf{e}^V$, $\mathcal{P}_\mathbf{e}^I(v)$, $\mathcal{P}_\mathbf{e}^V(v)$ & Summary of spatio-temporal invariant/variant patterns for each node\\ 
    $\mathbf{Z}^{1:t}$, $\mathbf{Z}_{\mathcal{P}_\mathbf{e}^I}^{1:t}$, $\mathbf{Z}_{\mathcal{P}_\mathbf{e}^V}^{1:t}$ & Summary of node representations, and their variants under  $\mathcal{P}_\mathbf{e}^I$ and $\mathcal{P}_\mathbf{e}^V$\\
    $\mathcal{S}_{\mathrm{ob}}$, $\mathcal{S}_{\mathrm{ge}}$ & Observed and generated environments sample libraries \\
    $s$, $\mathbf{s}_v$ & Intervention samples from $\mathcal{S}_{\mathrm{ob}}\cup\mathcal{S}_{\mathrm{ge}}$ and their summary for node $v$\\
    $\mathrm{do}(\cdot)$ & $do$-caculus for causal interventions\\
    $\mathcal{L}_\mathrm{task}$, $\mathcal{L}_\mathrm{risk}$, $\mathcal{L}_\mathrm{ECVAE}$ & Task loss, the invariance loss and the ECVAE loss\\
    $\alpha$, $\beta$ & Hyperparameters for loss trade-off\\
    
    \bottomrule
    \end{tabular}%
}
\vspace{-1em}
\end{table}%
