# Supplementary material for: GC-Bench: An Open and Unified Benchmark for Graph Condensation
Source: arXiv:2407.00615 source file (2024-11-21)
Supplement: Supplementary file 2 [file 1_algo.tex]

% algo box + comlexiety analysis
\section{Algorithm and Complexity Analysis}\label{sec:algorithm}
\setcounter{table}{0}
\setcounter{footnote}{0}
\setcounter{figure}{0}
\setcounter{equation}{0}

\IncMargin{1em}
\begin{algorithm}[h]
    \caption{Overall training process of \modelname.}
    \label{alg:alg}
    \KwIn{Dynamic graph $\mathbf{DG} = (\{ \mathcal{G} \}_{t=1}^{T})$ with labels $\mathbf{Y}^{1:T}$ of link occurrence; Number of training epochs $E$; Number of intervention times $S$; Hyperparameters $\alpha$ and $\beta$.}
    \KwOut{Optimized model $f_{\boldsymbol{\theta}}^{\star}$; Predicted label $Y^{T}$ of link occurrence at time $T+1$.}
    \BlankLine 
    Initialize parameters randomly\;
    \For{$i=1,2,\cdots,E$}{
         \vspace{0.5em}
        \tcp{Environments Modeling and Inferring} 
        Obtain representations for each node at each time with the support of $\mathbf{e}$, as $\mathbf{z}_{v}^{\mathbf{e},t} \gets$ Eq. \eqref{eq:repre}\;
        Establish the observed environment samples library $\mathcal{S}_{\mathrm{ob}} \gets$ Eq. \eqref{eq:sob}\;
        Infer the distribution $p_\omega(\mathbf{e})$ with $\mathcal{L}_{\mathrm{ECVAE}} \gets$ Eq. \eqref{eq:ecvae} and generate samples library $\mathcal{S}_{\mathrm{ge}}$\; \vspace{0.5em}
        % \BlankLine 
        \tcp{Environments Extrapolating} 
        Learn the invariance threshold $\delta_v \gets$ Eq. \eqref{eq:delta} by function $\mathbb{I}(\cdot) \gets$ Eq. \eqref{eq:trans}\;
        Recognize the invariant/variant patterns for each node, as $\mathcal{P}_\mathbf{e}^{I}(v)$, $\mathcal{P}_\mathbf{e}^{V}(v) \gets$ Eq. \eqref{eq:evi}\;
        Calculate task loss depending on the invariant patterns, as $\mathcal{L}_{\mathrm{task}} \gets$ Eq. \eqref{eq:taskloss}\;
        % \BlankLine 
         \vspace{0.5em}\tcp{Environments Generalizing}
        \For{$j=1,2,\cdots,S$}{
            Sample items from $\mathcal{S}_{\mathrm{ob}} \cup \mathcal{S}_{\mathrm{ge}}$ and perform intervention for each node, as Eq. \eqref{eq:intervention}\;
            Calculate intervention loss, as $\mathcal{L}_{\mathrm{risk}} \gets$ Eq. \eqref{eq:intervloss}\;
        }
         \vspace{0.5em}\tcp{Optimize}
        Calculate the overall loss, as $\mathcal{L} \gets$ Eq. \eqref{eq:final2}\;
        Update model parameters by minimizing $\mathcal{L}$.
    }
\end{algorithm}
\DecMargin{1em}
The overall training process of our \modelname~is shown is Algorithm~\ref{alg:alg}.

\textbf{Comlexity Analysis. }We analyze the computational complexity of each part in \modelname~as follows. Denote $|\mathcal{V}|$ and $|\mathcal{E}|$ as the total number of nodes and edges in each graph snapshot, respectively. 

In Section~\ref{sec:EIDyGNN}, operations of the EAConv layer in EA-DGNN can be parallelized across all nodes, which is highly efficient. Thus, the computation complexity of EA-DGNN is:
\begin{equation}\label{Eq:eadgnn}
    \mathcal{O} \left ( |\mathcal{E}| \sum_{l=0}^{L} d^{(l)} + \mathcal{V} \left ( \sum_{l=1}^{L} d^{(l-1)}d^{(l)} + (d^{(L)})^2 \right ) \right ),
\end{equation}
where $d^{(l)}$ denotes the dimension of the $l$-th layer. As $L$ is a small number, and $d^{(l)}$ is a constant, the Eq.~\eqref{Eq:eadgnn} can be rewritten as $\mathcal{O}(|\mathcal{E}|d+|\mathcal{V}|d^2)$, where $d$ is the universal notation of all $d^{(l)}$. 

In Section~\ref{sec:modeling}, the computation complexity of the ECVAE is a compound of the encoder and decoder, with the same computation complexity as $\mathcal{O}(|\mathbf{z}|Ld)$, where $|\mathbf{z}|$ is the number of the observed environment samples, $L$ is the number of layers in the encoder and decoder. Also, as $L$ is a small number, we omit it for brevity. Thus, the computation complexity of ECVAE is $\mathcal{O}(|\mathbf{z}|d)$. 

In Section~\ref{sec:invariant}, we recognize the invariant/variant patterns for all nodes by the function $\mathbb{I}(\cdot)$ in parallel, with the computation complexity $\mathcal{O}(K\log|\mathcal{V}|)$.

In Section~\ref{sec:optimize}, we perform sampling and replacing as an implementation of causal interventions. Denote $|\mathcal{E}|_p$ as the number of edges to predict and $|\mathcal{S}|$ as the size of the intervention set, which is usually set as a small constant. The spatio-temporal causal intervention mechanism owns a computation complexity compounding of sampling and replacing as $\mathcal{O}(|\mathcal{S}|d) + \mathcal{O}(|\mathcal{E}_p| |\mathcal{S}|d)$ in training, and no extra computation complexity in the inference stage.

Therefore, the overall computation complexity of \modelname~is:
\begin{equation}
    \mathcal{O}(|\mathcal{E}|d+|\mathcal{V}|d^2) + \mathcal{O}(|\mathbf{z}|d) + \mathcal{O}(K\log|\mathcal{V}|) + \mathcal{O}( |\mathcal{S}|d) + \mathcal{O}(|\mathcal{E}_p| |\mathcal{S}|d).
\end{equation}
In summary, \modelname~has a linear computation complexity with respect to the number of nodes and edges, which is on par with DIDA~\cite{zhang2022dynamic} and other existing dynamic GNNs. We believe that the computational complexity bottleneck of \modelname~lies in the spatio-temporal causal intervention mechanism. We further analyze the intervention efficiency in Appendix~\ref{sec:efficiency}.
