# Supplementary material for: GC-Bench: An Open and Unified Benchmark for Graph Condensation
Source: arXiv:2407.00615 source file (2024-11-21)
Supplement: Supplementary file 3 [file 4_experiments.tex]

\section{Experiment Details and Additional Results}\label{sec:exp}
\setcounter{table}{0}
\setcounter{footnote}{0}
\setcounter{figure}{0}
\setcounter{equation}{0}

\subsection{Datasets Details}\label{sec:datasets}

We use three real-world datasets to evaluate \modelname~on the challenging future link prediction task. 
\begin{itemize}[leftmargin=1.5em]
    \item \textbf{COLLAB}\footnote{\url{https://www.aminer.cn/collaboration}}~\cite{tang2012cross} is an academic collaboration dataset with papers that were published during 1990-2006 (16 graph snapshots). Nodes and edges represent authors and co-authorship, respectively. Based on the co-authored publication, there are five attributes in edges, including ``Data Mining'', ``Database'', ``Medical Informatics'', ``Theory'' and ``Visualization''. We pick ``Data Mining'' as the shifted attribute. We apply word2vec~\cite{mikolov2013efficient} to extract 32-dimensional node features from paper abstracts. We use 10/1/5 chronological graph snapshots for training, validation, and testing, respectively. The dataset includes 23,035 nodes and 151,790 links in total.
    \item \textbf{Yelp}\footnote{\url{https://www.yelp.com/dataset}}~\cite{sankar2020dysat} contains customer reviews on business. Nodes and edges represent customer/business and review behaviors, respectively. Considering categories of business, there are five attributes in edges, including ``Pizza'', ``American (New) Food'', ``Coffee~\&~Tea'', ``Sushi Bars'' and ``Fast Food'' from January 2019 to December 2020 (24 graph snapshots). We pick ``Pizza'' as the shifted attribute. We apply word2vec~\cite{mikolov2013efficient} to extract 32-dimensional node features from reviews. We use 15/1/8 chronological graph snapshots for training, validation, and testing, respectively. The dataset includes 13,095 nodes and 65,375 links in total.
    \item \textbf{ACT}\footnote{\url{https://snap.stanford.edu/data/act-mooc.html}}~\cite{kumar2019predicting} describes student actions on a MOOC platform within a month (30 graph snapshots). Nodes represent students or targets of actions, edges represent actions. Considering the attributes of different actions, we apply K-Means~\cite{hartigan1979algorithm} to cluster the action features into five categories and randomly select a certain category (the 5th cluster) of edges as the shifted attribute. We assign the features of actions to each student or target and expand the original 4-dimensional features to 32 dimensions by a linear function. We use 20/2/8 chronological graph snapshots for training, validation, and testing, respectively. The dataset includes 19,008 nodes and 202,339 links in total.
\end{itemize}
Statistics of the three datasets are concluded in Table~\ref{tab:datasets}. These three datasets have different time spans and temporal granularity (16 years, 24 months, and 30 days), covering most real-world scenarios. The most challenging dataset for the future link prediction task is the COLLAB. In addition to having the longest time span and the coarsest temporal granularity, it also has the largest difference in the properties of its links.
\begin{table}[htbp]
\caption{Statistics of the real-world datasets.}
\label{tab:data}
\centering
\resizebox{\linewidth}{!}{
    \begin{tabular}{ccccccc}
    \toprule
    \textbf{Dataset} & \textbf{\# Nodes} & \textbf{\# Links}  & \textbf{\makecell{\# Graph\\Snapshots}} & \textbf{\makecell{Temporal\\Granularity}}  & \textbf{In-distribution Attributes}& \textbf{\makecell{Shifted\\Attribute}} \\
    \midrule
    
    COLLAB & 23,035 & 151,790  & 16   & year & \makecell{Database, Medical Informatics,\\Theory, Visualization} & Data Mining\\
    \specialrule{0em}{1.2pt}{1.2pt}
    Yelp  & 13,095 & 65,375  & 24   & month  & \makecell{American (New) Food, Fast Food\\Sushi Bars, Coffee~\&~Tea} & Pizza\\
    \specialrule{0em}{1.2pt}{1.2pt}
    ACT   & 19,008 & 202,339  & 30   & day  & Attributes 1-4 & Attribute 5\\
    \bottomrule
    \end{tabular}%
}
\end{table}

We visualize the distribution shifts in the three real-world dataset with respect to the average neighbor degree (Figure~\ref{fig:degree}) and the number of interactions (Figure~\ref{fig:link}) in training and testing sets. We observe that, there exists a huge difference in terms of the values, trends, \etc, between the training set and the testing set, which demonstrates the distribution shifts are heavy. Interestingly, COLLAB has less testing data than its training data, which is common in real-world scenarios, such as not all the co-authorship was established from the beginning. In addition, we notice a drastic drop in Yelp after January 2019 when the COVID-19 outbreak. The sudden change in predictive patterns increases the difficulty of the task. A similar abnormal steep upward trend can also be witnessed in ACT after Day 20, which may be caused by an unknown out-of-distribution event.

\begin{figure}[htbp]
\centering
\subfigure[COLLAB]{
\includegraphics[width=0.33\linewidth]{fig/degree_collab.pdf}
\label{fig:de_collab}
}\hspace{-3mm} 
\subfigure[Yelp]{
\includegraphics[width=0.33\linewidth]{fig/degree_yelp.pdf}
\label{fig:de_yelp}
}\hspace{-3mm} 
\subfigure[ACT]{
\includegraphics[width=0.33\linewidth]{fig/degree_act.pdf}
\label{fig:de_act}
}
\centering
\caption{Visualizations of the average neighbor degree in each graph snapshot.}
\label{fig:degree}
\end{figure}

\begin{figure}[htbp]
\centering
\subfigure[COLLAB]{
\includegraphics[width=0.33\linewidth]{fig/links_collab.pdf}
\label{fig:link_collab}
}\hspace{-2.9mm} 
\subfigure[Yelp]{
\includegraphics[width=0.33\linewidth]{fig/links_yelp.pdf}
\label{fig:link_yelp}
}\hspace{-2.6mm} 
\subfigure[ACT]{
\includegraphics[width=0.33\linewidth]{fig/links_act.pdf}
\label{fig:link_act}
}
\centering
\caption{Visualizations of the number of interactions in each graph snapshot.}
\label{fig:link}
\end{figure}

\subsection{Baseline Details}

We compare \modelname~with representative GNNs and OOD generalization methods.
\begin{itemize}[leftmargin=1.5em]
    \item \textbf{Static GNNs}: 
    \textbf{GAE}~\cite{kipf2016variational} is a representative static GNN as the GCN~\cite{kipf2016semi} based graph autoencoder; \textbf{VGAE}~\cite{kipf2016variational} further introduces variational variables into GAE, possessing better generative ability.
    \item \textbf{Dynamic GNNs}: \textbf{GCRN}~\cite{seo2018structured} is a representative dynamic GNN following ``spatial first, temporal second'' convolution mechanism, which firstly adopts GCNs to obtain node embeddings and then a GRU~\cite{cho2014learning} to capture temporal relations; \textbf{EvolveGCN}~\cite{pareja2020evolvegcn} applies an LSTM~\cite{hochreiter1997long} or GRU to flexibly evolve the parameters of GCNs instead of modeling the dynamics after deriving node embeddings; \textbf{DySAT}~\cite{sankar2020dysat} models dynamic graph through self-attentions in both structural neighborhoods and temporal dynamics.
    \item \textbf{OOD generalization methods}: \textbf{IRM}~\cite{arjovsky2019invariant} minimizes the empirical risk to learn an optimal invariant predictor under potential environments; \textbf{V-REx}~\cite{krueger2021out} extends the IRM by reweighting the empirical risk to emphasize more on training samples with larger errors; \textbf{GroupDRO}~\cite{sagawa2019distributionally} reduces the empirical risk gap across training distributions to enhance the robustness when encountering heavy OOD shifts; \textbf{DIDA}~\cite{zhang2022dynamic} tackles OOD generalization problem on dynamic graphs for the first time by discovering and utilizing invariant patterns. It is worth noting that, DIDA is the most relative work as our main baseline for comparison.
\end{itemize}

\subsection{Experiment Setting Details}\label{sec:settings}

\textbf{Detailed Settings for Section~\ref{sec:exp1}. }
Each of the three real-world datasets can be split into several partial dynamic graphs based on their link properties, which demonstrates the multi-attribute relations under the impact of their surrounding environments. We filter out one certain attribute links as the variables under the future shifted environment as the OOD data, and the left links are further divided into training, validation, and testing sets chronologically. The shifted attribute links will only be accessible during the OOD testing stage, which is more practical and challenging in real-world scenarios as the model cannot capture any information about the filtered links during training and validation. Note that, all attribute-related features have been removed after the above operations before feeding to \modelname. Take the COLLAB dataset for example. There are five attribute links in COLLAB as summarized in Table~\ref{tab:datasets}. We filter out all the links with the attribute ``Data Mining'', and split the rest of the links into training, validation, and testing sets by positive and negative edge sampling. Then we add the ``Data Mining'' links into testing sets to make the distribution shifts. Finally, we remove all link attributes information to avoid data leakage.

\textbf{Detailed Settings for Section~\ref{sec:exp2}. }Denote original node features and structures as $\mathbf{X}^t \in \mathbb{R}^{N\times d}$ and $\mathbf{A}^t \in \{0,1\}^{N \times N}$. For each time $t$, we uniformly sample $p(t) | \mathcal{E}^{t+1} | $ positive links and $(1-p(t))| \mathcal{E}^{t+1}|$ negative links, which are then factorized into shifted features $\mathbf{X}^{t\prime} \in \mathbb{R}^{N \times d}$ while preserving structural property. Original node features and synthesized node features are concatenated as $[\mathbf{X}^t \| \mathbf{X}^{t\prime}]$ as the input. In details, $\mathbf{X}^{t\prime}$ is obtained by training the embeddings with reconstruction loss $\ell(\mathbf{X}^{t\prime} \mathbf{X}^{t\prime \top},\mathbf{A}^{t+1})$, where $\ell(\cdot)$ refers to the cross-entropy loss function~\cite{de2005tutorial}. In this way, we find that the link predictor can achieve satisfying results by using $\mathbf{X}^{t\prime} $ to predict the links in $\mathbf{A}^{t+1}$, which demonstrates that the generated node features have strong correlations with the future underlying environments. The sampling probability $p(t)=\bar{p}+\sigma \cos (t)$, where $\mathbf{X}^{t\prime} $ with higher $p(t)$ will have stronger spurious correlations with future underlying environments. Note that, we apply the $\mathrm{clip(\cdot)}$ function to limit the probability to between 0 and 1. We set $\bar{p}$ to be 0.4, 0.6 and 0.8 for training and 0.1 for testing; set $\sigma=$~0.05 in training and $\sigma=$~0 in testing.

\textbf{Detailed Settings for Section~\ref{sec:ipr}. }We set the number of nodes $N=$~2,000 with 10 graph snapshots, where 6/2/2 chronological snapshots are used for training, validation, and testing, respectively. We set $K=$~5 and let $\sigma_{\mathbf{e}}$ represent the proportion of the environments in which the invariant patterns are learned, where higher $\sigma_{\mathbf{e}}$ means more reliable invariant patterns. Node features with respect to different environments are drawn from five multivariate normal distributions $\mathcal{N}(\boldsymbol{\mu}_k;\boldsymbol{\sigma}_k)$. 
Features with respect to the invariant patterns will be perturbed slightly, while features with respect to the variant patterns will be perturbed significantly. Here we perturb features by adding Gaussian noise with different degrees. We then construct graph structures based on node feature similarity. Links generated by the node-pair representations under the $\mathbf{e}_{5}$ are filtered out during the training and validation stages, which is similar to the setting of Section~\ref{sec:exp1}, and they only appear in the testing stage following the proportion constraint $\bar{q}$. Higher $\bar{q}$ means more heavier distribution shifts. $\mathbb{I}_{\mathrm{ACC}}$ denotes the prediction accuracy of the invariant patterns by $\mathbb{I}(\cdot)$. As the environments $\mathbf{e}=\{\mathbf{e}_k\}_{k=1}^{5}$ do not satisfy the permutation invariance property, thus the predicted invariant patterns with respect to $\mathbf{e}$ is hard to evaluate. May wish to set the $\mathbb{I}_{\mathrm{ACC}}$ reports the highest results as we shift the orders of environments in $\mathbf{e}$ to satisfy the predicted invariant patterns better.

\subsection{Hyperparameter Sensitivity Analysis}\label{sec:sensitivity}
We analyze the sensitivity of the hyperparameters $\alpha$ and $\beta$, which act as the trade-off for loss in Eq.~\eqref{eq:final2}. The hyperparameter $\alpha$ is chosen from $\{ \text{10}^{-{\text3}},\text{10}^{-\text{2}},\text{10}^{-\text{1}},\text{10}^{\text{0}},\text{10}^{\text{1}} \}$, and $\beta$ is chosen from $\{ \text{10}^{-\text{6}}, \text{10}^{-\text{5}}, \text{10}^{-\text{4}}, \text{10}^{-\text{3}}, \text{10}^{-\text{2}} \}$. We conduct analysis on three real-world datasets and report results in Figure~\ref{fig:alpha} and Figure~\ref{fig:beta}. Results demonstrate that the task performance experiences a significant decline in most datasets when the values of $\alpha$ and $\beta$ are too large or too small. We can draw a conclusion that $\alpha$ acts as a balance factor between exploiting the spatio-temporal invariant patterns for out-of-distribution prediction and generalizing to diverse latent environments with respect to variant patterns. $\beta$ plays a role in balancing the trade-off between modeling the environment and inferring the environment distribution as a bi-level optimization. In conclusion, different combinations of hyperparameters lead to varying task performance, and we follow the tradition to report the best task performance with standard deviations.

\begin{figure}[htbp]
\centering
\subfigure[COLLAB]{
\includegraphics[width=0.32\linewidth]{fig/a_collab.pdf}
\label{fig:a_collab}
}\hspace{-2.5mm} 
\subfigure[Yelp]{
\includegraphics[width=0.32\linewidth]{fig/a_yelp.pdf}
\label{fig:a_yelp}
}\hspace{-2.5mm} 
\subfigure[ACT]{
\includegraphics[width=0.32\linewidth]{fig/a_act.pdf}
\label{fig:a_act}
}
\centering
\caption{Sensitivity analysis of the hyperparameter $\alpha$ on three real-world datasets. The solid line shows the average AUC (\%) in the testing stage and the light blue area represents standard deviations. The dashed line represents the average AUC (\%) of the best performed baseline.}
\label{fig:alpha}
\end{figure}

\begin{figure}[htbp]
\centering
\subfigure[COLLAB]{
\includegraphics[width=0.32\linewidth]{fig/b_collab.pdf}
\label{fig:b_collab}
}\hspace{-2.5mm} 
\subfigure[Yelp]{
\includegraphics[width=0.32\linewidth]{fig/b_yelp.pdf}
\label{fig:b_yelp}
}\hspace{-2.5mm} 
\subfigure[ACT]{
\includegraphics[width=0.32\linewidth]{fig/b_act.pdf}
\label{fig:b_act}
}
\centering
\caption{Sensitivity analysis of the hyperparameter $\beta$ on three real-world datasets. The solid line shows the average AUC (\%) in the testing stage and the light blue area represents standard deviations. The dashed line represents the average AUC (\%) of the best performed baseline.}
\label{fig:beta}
\end{figure}

\subsection{Intervention Efficiency Analysis}\label{sec:efficiency}
From the results of complexity analysis in Appendix~\ref{sec:algorithm}, we believe the computational complexity bottleneck of \modelname~lies in the spatio-temporal causal intervention mechanism. In this case, we analyze the intervention efficiency in the following two aspects.

\textbf{Intervention Ratio. }We perform node-wisely causal interventions as in Eq.~\eqref{eq:intervention}. However, executing interventions for all nodes in each epoch is time-consuming. Thus, we propose randomly selecting nodes and performing interventions according to a certain ratio. Let the intervention ratio represent the ratio of the number of intervened nodes to the total number of nodes $|\mathcal{V}|$. Figure~\ref{fig:sl} shows the changes in task performance (AUC \%) and the training time as the intervention ratio increases. We observe the AUC increases, proving that the spatio-temporal causal intervention mechanism is more effective in solving OOD generalization problem with more intervened nodes. In addition, we notice a jump in the growth rate of AUC on three datasets at the ratio of 0.6, which indicates the most suitable intervention ratio while maintaining an acceptable training time cost.

\textbf{Mixing Ratio. }The intervention set $\mathbf{s}_v$ is sampled from $\mathcal{S}_{\mathrm{ob}}\cup \mathcal{S}_{\mathrm{ge}}$. While $\mathcal{S}_{\mathrm{ob}}$ has been already prepared after we model the environments in Section~\ref{sec:EIDyGNN}, the $\mathcal{S}_{\mathrm{ge}}$ requires instantly generating, which may be a burden on the intervention efficiency. Let the maxing ratio represent the ratio of the number of observed environment samples to the number of generated environment samples. Figure~\ref{fig:hh} shows the changes in task performance (AUC \%) and the training time as the mixing ratio increases. Different from the trend in Figure~\ref{fig:sl}, AUC reached the maximum value at different ratios on the three datasets, and when the ratio is too large or small, the model performs poorly, indicating that different datasets have varying preferences for mixing ratio settings. In addition, we observe the variation in training time is not significant, verifying that although $\mathcal{S}_{\mathrm{ob}}$ needs to be generated instantly, its time cost is acceptable still, and we should pay more attention on the optimal mixing ratio.

\begin{figure}[htbp]
\centering
\subfigure[COLLAB]{
\includegraphics[width=0.33\linewidth]{fig/collab_shuliang.pdf}
\label{fig:sl_collab}
}\hspace{-3mm} 
\subfigure[Yelp]{
\includegraphics[width=0.33\linewidth]{fig/yelp_shuliang.pdf}
\label{fig:sl_yelp}
}\hspace{-3mm} 
\subfigure[ACT]{
\includegraphics[width=0.33\linewidth]{fig/act_shuliang.pdf}
\label{fig:sl_act}
}
\centering
\caption{Intervention efficiency analysis on the intervention ratio. The vertical dashed line indicates the most suitable intervention ratio while maintaining an acceptable training time cost.}
\label{fig:sl}
\end{figure}

\begin{figure}[htbp]
\centering
\subfigure[COLLAB]{
\includegraphics[width=0.33\linewidth]{fig/collab_hunhe.pdf}
\label{fig:hh_collab}
}\hspace{-3mm} 
\subfigure[Yelp]{
\includegraphics[width=0.33\linewidth]{fig/yelp_hunhe.pdf}
\label{fig:hh_yelp}
}\hspace{-3mm} 
\subfigure[ACT]{
\includegraphics[width=0.33\linewidth]{fig/act_hunhe.pdf}
\label{fig:hh_act}
}
\centering
\caption{Intervention efficiency analysis on the mixing ratio. The vertical dashed line indicates the ratio when AUC reached the maximum value.}
\label{fig:hh}
\end{figure}

\subsection{Additional Analysis of Section~\ref{sec:rq1}}
We visualize Table 1 and Table 2 in Section 4.1 to provide additional analysis. We have concluded in Section~\ref{sec:rq1} that the baselines own a strong fitting ability but weak generalization ability between the distribution shifts settings. In addition to visualizing the task performance (AUC \%) under \textit{w/o OOD} and \textit{w/ OOD} settings, Figure~\ref{fig:delta_add} annotates the decrease of AUC under each baseline method, where the horizontal dashed line represents the AUC decrease of our \modelname. The smaller the decrease, the stronger the control ability under the impact of out-of-distribution shifts. We can observe that on the vast majority of datasets, our method can improve task performance in both \textit{w/o OOD} and \textit{w/ OOD} scenarios while minimizing AUC decrease. Our control over AUC decrease exceeds the baseline except for GAE and GCRN in the vast majority of cases. For the above two baseline methods, although they have better control ability over AUC decrease than our method, the premise is that their task performance is inherently poor. In addition, our method achieves the most excellent task performance on the ACT dataset, which can explain the unsatisfying but acceptable AUC decrease control. In summary, in addition to evaluating the advantages of our \modelname~in terms of task performance and generalization ability, which is the most topic-relative and common, our \modelname~also maintains the ability to reduce the impact of OOD on task performance.

\begin{figure}[htbp]
\centering
\subfigure[COLLAB]{
\includegraphics[width=0.33\linewidth]{fig/delta_collab.pdf}
\label{fig:delta_collab_link}
}\hspace{-3mm} 
\subfigure[Yelp]{
\includegraphics[width=0.33\linewidth]{fig/delta_yelp.pdf}
\label{fig:delta_yelp_link}
}\hspace{-3mm} 
\subfigure[ACT]{
\includegraphics[width=0.33\linewidth]{fig/delta_act.pdf}
\label{fig:delta_act_link}
}\\
\subfigure[COLLAB ($\bar{p}=$~0.4)]{
\includegraphics[width=0.33\linewidth]{fig/delta_collab_1.pdf}
\label{fig:delta_collab_n1}
}\hspace{-3mm} 
\subfigure[COLLAB ($\bar{p}=$~0.6)]{
\includegraphics[width=0.33\linewidth]{fig/delta_collab_2.pdf}
\label{fig:delta_collab_n2}
}\hspace{-3mm} 
\subfigure[COLLAB ($\bar{p}=$~0.8)]{
\includegraphics[width=0.33\linewidth]{fig/delta_collab_3.pdf}
\label{fig:delta_collab_n3}
}
\centering
\caption{Additional analysis of the performance on future link prediction.}
\label{fig:delta_add}
\end{figure}

\subsection{Additional Results of Section~\ref{sec:ipr}}
\label{sec:ipr_add}

Section~\ref{sec:ipr} reports the results when $\bar{q}=$~0.8. Here we report the additional results when $\bar{q}=$~0.4 and 0.6 in Figure~\ref{fig:syn_add}. All detailed results are summarized in Table~\ref{haha}. A similar trend can be observed as we report in Section~\ref{sec:ipr} that as $\sigma_{\mathbf{e}}$ increases, the performance of \modelname~shows a significant increase while narrowing the gap between \textit{w/o OOD} and \textit{w/ OOD} scenarios. Although DIDA also shows an upward trend, its growth rate is much more gradual, which indicates that DIDA is difficult to perceive changes in the underlying environments caused by different $\sigma_{\mathbf{e}}$ as it is incapable of modeling the environments, thus cannot achieve satisfying generalization performance. In addition, we also notice a positive correlation between $\mathbb{I}_{\mathrm{ACC}}$ and the AUC, which verifies the improvements are attributed to the proper recognition of the invariant patterns by $\mathbb{I}(\cdot)$. In conclusion, our \modelname~can exploit more reliable invariant patterns, thus performing high-quality invariant learning and efficient causal interventions, and achieving better generalization ability.

\begin{figure}[htbp]
\centering
\subfigure[$\bar{q}=$~0.4]{
\includegraphics[width=0.48\linewidth]{fig/synthetic_0.4.pdf}
\label{fig:syn_0.4}
}
\subfigure[$\bar{q}=$~0.6]{
\includegraphics[width=0.48\linewidth]{fig/synthetic_0.6.pdf}
\label{fig:syn_0.6}
}
\centering
\caption{Additional results on the effects of invariant pattern recognition.}
\label{fig:syn_add}
\end{figure}

\input{table/addition_syn}
