# Supplementary material for: GC-Bench: An Open and Unified Benchmark for Graph Condensation
Source: arXiv:2407.00615 source file (2024-11-21)
Supplement: Supplementary file 4 [file 5_implementation_details.tex]

\section{Implementation Details}\label{sec:imp}
\setcounter{table}{0}
\setcounter{footnote}{0}
\setcounter{figure}{0}
\setcounter{equation}{0}

\subsection{Training and Evaluation}
\textbf{Training Settings. }The number of training epochs for optimizing our proposed method and all baselines is set to 1000. We adopt the early stopping strategy, \ie, stop training if the performance on the validation set does not improve for 50 epochs. For our \modelname, the hyperparameter $\alpha$ is chosen from $\{ \text{10}^{-{\text3}},\text{10}^{-\text{2}},\text{10}^{-\text{1}},\text{10}^{\text{0}},\text{10}^{\text{1}} \}$, and $\beta$ is chosen from $\{ \text{10}^{-\text{6}}, \text{10}^{-\text{5}}, \text{10}^{-\text{4}}, \text{10}^{-\text{3}}, \text{10}^{-\text{2}} \}$. The intervention ratio and the mixing ratio are carefully tuned for each dataset. For other parameters, we adopt the Adam optimizer~\cite{kingma2014adam} with an appropriate learning rate and weight decay for each dataset and adopt the grid search for the best performance using the validation split. All parameters are randomly initiated, which is especially important for $\mathbf{W}_k$ in Eq.~\eqref{eq:proj} that ensures the difference in each environment embedding space. The $K$ channels will still remain orthogonal during training as we conduct discrete environment disentangling iteratively. This helps the recognition of invariant/variant patterns mainly because we guarantee there is no overlap between environments.

\textbf{Evaluation. }According to respective experiment settings, we randomly split the dynamic datasets into training, validation, and testing chronological sets. We sample negative links from nodes that do not have links, and the negative links for validation and testing sets are kept the same for all baseline methods and ours. We set the number of positive links to the same as the negative links. We use the Area under the ROC Curve (AUC)~\cite{bradley1997use} as the evaluation metric. As we focus on the future link prediction task, we use the inner product of a pair of learned node representations to predict the occurrence of links, \ie, we implement the link predictor $g(\cdot)$ as the inner product of hidden embeddings, which is commonly applied in classic future link prediction tasks. The biased training technique is adopted following~\cite{cadene2019rubi}. We use the cross-entropy loss as the loss function $\ell(\cdot)$. The activation function is LeakyReLU~\cite{agarap2018deep}. We randomly run all the experiments five times, and report the average results with standard deviations.

\subsection{Baseline Implementation Details} 

We provide the baseline methods implementations with respective licenses as follows.
\begin{itemize}[leftmargin=1.5em]
    \item {GAE}~\cite{kipf2016variational}: \url{https://github.com/DaehanKim/vgae_pytorch} with MIT License.
    \item {VGAE}~\cite{kipf2016variational}: \url{https://github.com/DaehanKim/vgae_pytorch} with MIT License.
    \item {GCRN}~\cite{seo2018structured}: \url{https://github.com/youngjoo-epfl/gconvRNN} with MIT License.
    \item {EvolveGCN}~\cite{pareja2020evolvegcn}: \url{https://github.com/IBM/EvolveGCN} with Apache-2.0 License.
    \item {DySAT}~\cite{sankar2020dysat}: \url{https://github.com/FeiGSSS/DySAT_pytorch} with license unspecified.
    \item {IRM}~\cite{arjovsky2019invariant}: \url{https://github.com/facebookresearch/InvariantRiskMinimization} with CC BY-NC 4.0 License.
    \item {V-REx}~\cite{krueger2021out}: \url{https://github.com/capybaralet/REx_code_release} with license unspecified.
    \item {GroupDRO}~\cite{sagawa2019distributionally}: \url{https://github.com/kohpangwei/group_DRO} with MIT License.
    \item {DIDA}~\cite{zhang2022dynamic}: \url{https://github.com/wondergo2017/DIDA} with license unspecified.
\end{itemize}
The parameters of baseline methods are set as the suggested value in their papers or carefully tuned for fairness.

\subsection{Configurations}
We conduct the experiments with:
\begin{itemize}[leftmargin=1.5em]
    \item Operating System: Ubuntu 20.04 LTS.
    \item CPU: Intel(R) Xeon(R) Platinum 8358 CPU@2.60GHz with 1TB DDR4 of Memory.
    \item GPU: NVIDIA Tesla A100 SMX4 with 40GB of Memory.
    \item Software: CUDA 10.1, Python 3.8.12, PyTorch~\cite{paszke2019pytorch} 1.9.1, PyTorch Geometric~\cite{fey2019fast} 2.0.1.
\end{itemize}
