# Supplementary material for: GC-Bench: An Open and Unified Benchmark for Graph Condensation
Source: arXiv:2407.00615 source file (2024-11-21)
Supplement: Supplementary file 5 [file 6_furthur_discussions.tex]

\section{Further Discussions}\label{sec:further}
\setcounter{table}{0}
\setcounter{footnote}{0}
\setcounter{figure}{0}
\setcounter{equation}{0}

\subsection{Further Analysis on SCM Model}\label{sec:scm}

We provide further analysis of the intrinsic cause of the out-of-distribution shifts. From the causal-based theories~\cite{pearl2009causal, pearl2010causal,pearl2018book}, we formulate the generation process of static graphs and dynamic graphs with the Structural Causal Model (SCM)~\cite{pearl2009causal} in Figure~\ref{fig:scm_appendix}, where the arrow between variables denotes causal dependencies. It is widely accepted in the OOD generalization works~\cite{gagnon2022woods, arjovsky2019invariant, rosenfeld2020risks, wu2022discovering, chang2020invariant, ahuja2020invariant, mitrovic2020representation} that the correlations between labels and certain parts of the latent features are invariant across data distributions in training and testing, while the other parts of the features are variant. The invariant part is also called the causal part ($C$) and the variant part is also called the spurious part ($S$). 

\textbf{Qualitative Analysis. }In the SCM model on static graphs, $C$ \tikz[baseline=-0.7ex]{\draw[->] (0,0) -- (0.3,0);} $\mathbf{G}$  \tikz[baseline=-0.7ex]{\draw[<-] (0,0) -- (0.3,0);} $S$ demonstrates that the invariant part and variant part jointly decide the generation of the graphs, while $C$ \tikz[baseline=-0.7ex]{\draw[->] (0,0) -- (0.3,0);} $\mathbf{Y}$ denotes the label is solely determined by the causal part. However, there exists the spurious correlation $C$\tikz[baseline=-0.7ex]{\draw[dashed, <->] (0,0) -- (0.6,0);}$S$ in certain distributions that would lead to a backdoor causal path $S$ \tikz[baseline=-0.7ex]{\draw[dashed, ->] (0,0) -- (0.4,0);} $C$ \tikz[baseline=-0.7ex]{\draw[->] (0,0) -- (0.3,0);} $\mathbf{Y}$ so that the variant part and the label are correlated statistically. As the variant part changes in the testing distributions caused by different environments $\mathbf{e}$, the predictive patterns built on the spurious correlations expired. For the same reason, similar spurious correlation $C^t$\tikz[baseline=-0.7ex]{\draw[dashed, <->] (0,0) -- (0.6,0);}$S^t$ exists on dynamic graphs within a single graph snapshot, which opens the backdoor causal path $S^{t}$ \tikz[baseline=-0.7ex]{\draw[dashed, ->] (0,0) -- (0.4,0);} $C^{t}$ \tikz[baseline=-0.7ex]{\draw[->] (0,0) -- (0.3,0);} $\mathbf{Y}^{t}$. Especially, as we have captured the temporal dynamics between each graph snapshot, the variant part in the previous time slice may also establish spurious correlations with the invariant part at present time, \ie, $C^{t-1}$\tikz[baseline=-0.7ex]{\draw[dashed, <->] (0,0) -- (0.6,0);}$S^t$, leading to $S^{t-1}$ \tikz[baseline=-0.7ex]{\draw[dashed, ->] (0,0) -- (0.4,0);} $C^t$ \tikz[baseline=-0.7ex]{\draw[->] (0,0) -- (0.3,0);} $\mathbf{Y}^t$, which is a unique phenomenon in the dynamic scenarios. Hence, we propose to get rid of the spurious correlations within and between graph snapshots by investigating the latent environment variable $\mathbf{e}$, encouraging the model to rely on the spatio-temporal invariant patterns to make predictions, and thus handle the distribution shifts.

\textbf{Further Analysis of Assumption 1. }The causal inference theories~\cite{pearl2009causal, pearl2010causal, pearl2018book} propose to get rid of the spurious correlations by blocking the backdoor path with $do$-calculus, which would remove all causal dependencies on the intervened variables. Particularly, we intervene the variant parts on all graph snapshots, \ie, $\mathrm{do}(S^{t})$, and thus the spurious correlations within and between graph snapshots can be filtered out. This encourages the two conditions in Assumption 1 to be satisfied: the Invariance Property will be satisfied if the spurious correlations $S^{t-1}$\tikz[baseline=-0.7ex]{\draw[dashed, <->] (0,0) -- (0.6,0);\draw[red] (0.2,0.1) -- (0.4,-0.1);\draw[red] (0.4,0.1) -- (0.2,-0.1);}$C^t$\tikz[baseline=-0.7ex]{\draw[dashed, <->] (0,0) -- (0.6,0);\draw[red] (0.2,0.1) -- (0.4,-0.1);\draw[red] (0.4,0.1) -- (0.2,-0.1);}$S^t$ are removed and the label will be solely decided by the invariant part $C^t$ \tikz[baseline=-0.7ex]{\draw[->] (0,0) -- (0.3,0);} $\mathbf{Y}^t$, which also satisfies the Sufficient Condition. In this case, we can minimize the variance of the empirical risks under diverse potential environments, while encouraging the model to make predictions of the spatio-temporal invariant patterns.

\textbf{Further Explanations of the Toy Example. }From the above analysis, we can further explain the toy example in Figure 1(a). The prediction model has captured the spurious correlations between ``coffee'' and the ``cold drink'', which caused the false prediction of buying an Iced Americano in the winter. By applying our environment-ware \modelname, the prediction model can perceive the environments of seasons through the neighbors around the central node, \ie, perceiving the winter season by learning the observed interactions between the user and the thick clothing. Thus encouraging the model to rely on the exploited spatio-temporal invariant patterns, \ie, ``the user buys coffee'', to make the correct prediction on the Hot Latte by considering underlying environments.
\vspace{-0.5em}

\begin{figure}[h]
    \centering
    \includegraphics[width=0.7\linewidth]{fig/scm_appendix.pdf}
    \vspace{-0.5em}
    \caption{The SCM model on static graphs and dynamic graphs. }
    \label{fig:scm_appendix}
\end{figure}

\subsection{Further Related Work}\label{sec:related_work}

\textbf{Dynamic Graph Learning.} Extensive research~\cite {roddick1999bibliography, atluri2018spatio} address the challenges of learning on dynamic graphs, which consist of multiple graph snapshots at different times. Dynamic graph neural networks (DGNNs) are widely adopted to learn dynamic graphs by intrinsically modeling both spatial and temporal patterns, which can be divided into two main categories: spatial-first methods and temporal-first methods. The spatial-first methods~\cite{yang2021discrete, hajiramezanali2019variational, seo2018structured} first adopt vanilla GNNs to model spatial patterns for each graph snapshot, followed by sequential-based models like RNNs~\cite{medsker2001recurrent} or LSTMs~\cite{hochreiter1997long}, to capture temporal relations. In comparison, temporal-first DGNNs~\cite{wang2021inductive, rossi2020temporal} model dynamics in advance with temporal encoding mechanisms~\cite{hu2020heterogeneous}, and then conduct convolutions of message-passing and aggregating on each single graph with GNNs. Dynamic graph learning has been widely utilized for prediction tasks like disease transmission prediction~\cite{kapoor2020examining}, dynamic recommender system~\cite{you2019hierarchical}, social relation prediction~\cite{wang2021tedic}, \etc~However, most existing works fail to generalize under distribution shifts.
DIDA~\cite{zhang2022dynamic} is the sole prior work that addresses distribution shifts on dynamic graphs with an intervention mechanism. But DIDA neglects to model the complex environments on dynamic graphs, which is crucial in tackling distribution shifts. We also experimentally validate the advantage of our method compared with DIDA. 

\textbf{Out-of-Distribution Generalization.} Most machine learning methods are built on the I.I.D. hypothesis, \ie, training and testing data follow the independent and identical distribution, which can hardly be satisfied in real-world scenarios~\cite{shen2021towards}, as the generation and collection process of data are affected by many latent factors~\cite{rojas2018invariant, arjovsky2019invariant}. The non-I.I.D. distribution results in a significant decline of model performance, highlighting the urgency to investigate generalized learning methods for out-of-distribution (OOD) shifts, especially for high-stake downstream applications, like  autonomous driving~\cite{dai2018dark}, financial system~\cite{pareja2020evolvegcn}, \etc~OOD generalization has been extensively studied in both academia and industry covering various areas~\cite{shen2021towards, yuan2022towards, hendrycks2021many} and we mainly focus on OOD generalization on graphs~\cite{li2022out}. Most graph-targeted works concentrate on node-level or graph-level tasks on static graphs~\cite{zhu2021shift, fan2021generalizing, li2022ood, wu2022handling, li2022learning, chen2022learning, wu2022discovering}, targeting at solving the problems of graph OOD generalization for drugs, molecules, \etc, which is identified as one key challenge in AI for science (AI4Science). Another main category of works elaborates systematic benchmarks for graph OOD generalization evaluation~\cite{gui2022good, ding2021closer, ji2022drugood}. However, there lack of further research on dynamic graphs with more complicated shift patterns caused by spatio-temporal varying latent environments, which is our main concern.

\textbf{Invariant Learning.} Deep learning models tend to capture predictive correlations behind observed samples, while the learned patterns are not always consistent with in-the-wild extrapolation. Invariant learning aims to exploit the less variant patterns that lead to informative and discriminative representations for stable prediction~\cite{creager2021environment, li2021learning, zhao2019learning}. Supporting by disentangled learning theories and causal learning theories, invariant learning tackles the OOD generalization problem from a more theoretical perspective, revealing a promising power. Disentangle-based methods~\cite{bengio2013representation, locatello2019challenging} learn representations by separating semantic factors of variations in data, making it easier to distinguish invariant factors and establish reliable correlations. Causal-based methods~\cite{gagnon2022woods, arjovsky2019invariant, rosenfeld2020risks, wu2022discovering, chang2020invariant, ahuja2020invariant, mitrovic2020representation} utilize Structural Causal Model (SCM)~\cite{pearl2009causal} to filter out spurious correlations by intervention or counterfactual with $do$-calculus~\cite{pearl2010causal, pearl2018book} and strengthen the invariant causal patterns. However, the invariant learning method of node-level tasks on dynamic graphs is underexplored, mainly due to its complexity in analyzing both spatial and temporal invariant patterns.
