# Supplementary material for: GC-Bench: An Open and Unified Benchmark for Graph Condensation
Source: arXiv:2407.00615 source file (2024-11-21)
Supplement: Supplementary file 6 [file more.tex]

Note that, $f_{\boldsymbol{\theta}}$ relies on the $\mathcal{G}^{1:T}_{\mathbf{e}_I}$ to make predictions in the expectation term, while it depend on the complete representations $\mathcal{G}^{1:T}$ after intervening the $\mathcal{G}^{1:T}_{\mathbf{e}_V}$ to predict and calcute variance.

 \begin{itemize}[leftmargin=1.5em]
    \item Static GNNs: \textbf{GAE}~\cite{} is a representative static GNN as a GCN~\cite{} based graph autoencoder; \textbf{VGAE}~\cite{} further introduces variational variables into GAE, possessing better generative ability.
    \item Dynamic GNNs: \textbf{GCRN}~\cite{} is a representative dynamic GNN following ``spatial first, temporal second'' mechanism, which firstly adopts GCNs to obtain node embeddings and then a GRU~\cite{} to capture temporal relations; \textbf{EvolveGCN}~\cite{} applies an LSTM~\cite{} or GRU to flexibly evolve the parameters of GCNs, instead of modeling the dynamics after deriving node embeddings; \textbf{DySAT}~\cite{} models dynamic graph through self-attentions in both structural neighborhoods and temporal dynamics.
    \item OOD generalization methods: \textbf{IRM}~\cite{} minimizes the empirical risk to learn an optimal invariant predictor under potential environments; \textbf{V-REx} extends the IRM by reweighting the empirical risk to emphasize more on training samples with larger errors; \textbf{GroupDRO}~\cite{} reduces the empirical risk gap across training distributions to enhance the robustness when encountering heavy OOD shifts; \textbf{DIDA}~\cite{} tackles OOD generalization problem on dynamic graphs for the first time by discovering and utilizing invariant patterns. It is worth noting that, DIDA is the most relative work as our main baseline for comparison.
\end{itemize}

\begin{itemize}[leftmargin=1.5em]
    \item \textbf{COLLAB}~\cite{} is an academic collaboration dataset with papers that were published during 1990-2006. Nodes and edges represent authors and coauthorship, respectively. Based on the co-authored publication, there are five attributes in edges, including \texttt{Data Mining}, \texttt{Database}, \texttt{Medical Informatics}, \texttt{Theory} and \texttt{Visualization}. We pick \texttt{Data Mining} as the shifted variables.
    \item \textbf{Yelp}~\cite{} contains customer reviews on business. Nodes and edges represent customer/business and review behaviors, respectively. Considering categories of business, there are five attribute in edges, including \texttt{Pizza}, \texttt{American (New) Food}, \texttt{Coffee~\&~Tea}, \texttt{Sushi Bars} and \texttt{Fast Food} from January 2019 to December 2020. We pick \texttt{Pizza} as the shifted variables. 
    \item \textbf{ACT}~\cite{} describes students actions on a MOOC platform. Nodes represent students or targets of actions, edges represent actions. Considering the attributes of different actions, we apply K-Means~\cite{} to cluster the action features into five categories and randomly select a certain category of edges as the shifted variables.
\end{itemize}

\textbf{Settings.} %Each dataset can be split into several partial dynamic graphs based on their link properties, demonstrating the multi-attribute relations under the impact of surrounding environments. 
We filter out a certain attribute links as the variables under the future shifted environment as the OOD data, and the left are further divided into training, validation and testing sets chronologically. The shifted attribute links will only be accessible during OOD validation and testing. \zwmask{,which is more practical and challenging in the real-world scenarios as the model cannot capture any information about the filtered links during training. Note that, all attribute-related features have been removed after the above operations before feeding to \modelname.}

\textbf{Dynamic Graph Learning.} Extensive researches~\cite{roddick1999bibliography, atluri2018spatio} address the challenges of learning on dynamic graphs, which consist multiple snapshots in different times. Dynamic graph neural networks (DGNNs) intrinsically model both spatial and temporal patterns, which can be divided into two main categories: spatial-first and temporal-first methods~\cite{li2022autost}. The spatial-first methods~\cite{yang2021discrete, sun2021hyperbolic, hajiramezanali2019variational, seo2018structured} first adopt vanilla GNNs~\cite{} to model spatial patterns for each graph snapshot, followed by sequential-based models like RNNs~\cite{} or LSTMs~\cite{}, to capture temporal relations. In comparison, temporal-first DGNNs~\cite{wang2021inductive, rossi2020temporal} model dynamics in advance with temporal encoding mechanisms~\cite{hu2020heterogeneous}, and then conduct message-passing and aggregating on graphs with GNNs. \zwmask{Dynamic graph learning has been widely used for prediction tasks like disease transmission prediction~\cite{kapoor2020examining}, dynamic recommender system~\cite{you2019hierarchical}, social relation prediction~\cite{wang2021tedic}, \etc.} However, most existing works fail to generalize under distribution shifts.
\zw{DIDA is the sole prior work that tackles distribution shifts on dynamic graphs with an intervention mechanism. But DIDA neglects modeling the complex environments on dynamic graphs, which is crucial in tackling distribution shifts. We also experimentally validate the advantage of our method compared with DIDA. }

\textbf{Out-of-Distribution Generalization.} Most of machine learning methods are built on the I.I.D. hypothesis, \ie, training and testing data follow the independent and identical distribution, which can hardly be satisfied in real-world scenarios~\cite{shen2021towards}, as the generation and collection process of data are affected by many latent factors~\cite{rojas2018invariant, arjovsky2019invariant}. The non-I.I.D. distribution results in a significant decline of model performance, highlighting the urgency to investigate generalized learning method for out-of-distribution (OOD) shifts, especially for high-stake downstream applications, like  autonomous driving~\cite{dai2018dark}, financial system~\cite{pareja2020evolvegcn}, \etc. OOD generalization has been extensively studied in both academia and industry covering various areas~\cite{shen2021towards, yuan2022towards, hendrycks2021many} and we mainly focus on graphs~\cite{li2022out}. Most graph-targeted works concentrate on static graphs for node-level or graph-level tasks~\cite{zhu2021shift, fan2021generalizing, li2022ood, wu2022handling, li2022learning, chen2022learning, wu2022discovering}. Another category of works elaborate systematic benchmarks for graph OOD generalization evaluation~\cite{gui2022good, ding2021closer, ji2022drugood}. However, there lacks further research on dynamic graphs~\cite{zhang2022dynamic} with more complicated shift patterns caused by time-varying latent environments, which is our main concern.

\textbf{Invariant Learning.} Deep learning models tend to capture predictive correlations behind observed samples, while the learned patterns are not always consistent with in-the-wild extrapolation. Invariant learning aims to exploit the invariant patterns that leads to stable and informative representations for predicting~\cite{creager2021environment, li2021learning, zhao2019learning}. Supporting by disentangled learning~\cite{} and causal learning~\cite{} theories, invariant learning addresses OOD generalization problem from a more theoretical perspective, revealing a promising power. Disentangle-based methods learn representations by separating semantic factors of variations in data~\cite{bengio2013representation, locatello2019challenging}, making it easier to distinguish invariant factors and establishing reliable correlations. Causal-based methods utilize Structural Causal Model (SCM)~\cite{pearl2009causal} to filter spurious correlations by intervention or counterfactual with $do$-calculus~\cite{pearl2010causal, pearl2018book} and strengthen the invariant causal patterns.

\textbf{Environment Instantiation Mechanism.} We replace the environment instantiation mechanism in Section \ref{sec:modeling} by carrying out interventions only with observed environment samples (denoted as \textit{w/o EI}). We can see from Figure \ref{fig:abla} that the performance consistently drops, which validates that the environment instantiation mechanism help the model to generalize.

\textbf{Invariant Pattern Recognition Mechanism.} We replace the the invariant function $\mathbb{I}(\cdot)$ in Section \ref{sec:invariant} by determining the time-invariant patterns set randomly for each node (denoted as \textit{w/o IPR}). From Figure \ref{fig:abla}, we can observe a more severe decline with an average drop in AUC by 4.5\%, especially on ACT and COLLAB ($\bar{p}=$~0.6). Without the superiority of $\mathbb{I}(\cdot)$, the model cannot recognize the time-invariant patterns, thus the effectiveness of causal intervention later has been reduced.

\textbf{Intervention Mechanism.}  We remove the intervention mechanism in Section \ref{sec:optimize} and directly optimize the model by Eq. \eqref{eq:final2} without the $\mathcal{L}_{\mathrm{risk}}$ term (denoted as \textit{w/o Interv}). From Figure \ref{fig:abla}, we observe an average decline of 9.1\%, making the model degrade to the dynamic GNNs baselines approximately. This implies the indispensability of the intervention mechanism.
