# Supplementary material for: GC-Bench: An Open and Unified Benchmark for Graph Condensation
Source: arXiv:2407.00615 source file (2024-11-21)
Supplement: Supplementary file 7 [file relatedwork.tex]

\section{Summary of GC Methods}

% Please add the following required packages to your document preamble:
% \usepackage{multirow}
% \usepackage[table,xcdraw]{xcolor}
% Beamer presentation requires \usepackage{colortbl} instead of \usepackage[table,xcdraw]{xcolor}
% \usepackage[normalem]{ulem}
% \useunder{\uline}{\ul}{}
