# Supplementary material for: GC-Bench: An Open and Unified Benchmark for Graph Condensation
Source: arXiv:2407.00615 source file (2024-11-21)
Supplement: Supplementary file 8 [file GC_package.tex]

\section{Package}
We have developed a open-sourced package \todo{XXX}, which offers a comprehensive and unbiased platform for evaluating graph condensation methods and facilitating future research in this domain. 
